# Supplementary material for: RevSAM2: Prompt SAM2 for Medical Image Segmentation via Reverse-Propagation without Fine-tuning
Source: arXiv:2409.04298 source file (2024-11-25)
Supplement: Supplementary file 1 [file X_suppl.tex]

% \clearpage
\appendix
% \maketitlesupplementary

\begin{center}
{\centering\Large\bf RevSAM2: Prompt SAM2 for Medical Image Segmentation via Reverse-Propagation without Fine-tuning} 
\textbf{}\\
\vspace{0.5em}\Large Supplementary Material \\
\vspace{1.0em}
\end{center}

\setcounter{section}{0}

% In the supplementary material, we provide the details of comparisons with other few-shot methods (Sec \ref{sec:sup_few_shot}), qualitative results (Sec \ref{sec:qualitative}), and detailed results of the three support groups we used (Sec \ref{sec:supp_detail_results}).

\section{Comparison with Few-Shot Methods}
\label{sec:sup_few_shot}

In Table 4 in the main paper, we compare RevSAM2 with other few-shot methods \cite{aasdcl,srcl,rpt,GMRD}. As shown in Fig. \ref{fig:comp_few_shot} in the supplementary material, these methods process each slice (\emph{e.g.}, $\textbf{\textit{q}}_1$, $\textbf{\textit{q}}_2$,...) in the query volume $\textbf{\textit{Q}}$ individually by inputting it into the network along with the support image $\textbf{\textit{S}}$ and its mask $\textbf{\textit{Y}}$ (Fig \ref{fig:comp_few_shot} (a)), without considering information from adjacent slices in the query volume. For RevSAM2 experiments, we stack the query slices corresponding to the same support image (Fig \ref{fig:comp_few_shot} (b)). It is important to note that we strictly adhere to the selection strategy for support and query images used by other methods to ensure a fair comparison.\vspace{-0.5em}

\begin{figure}[htbp]
\centering
\includegraphics[width=0.6\linewidth]{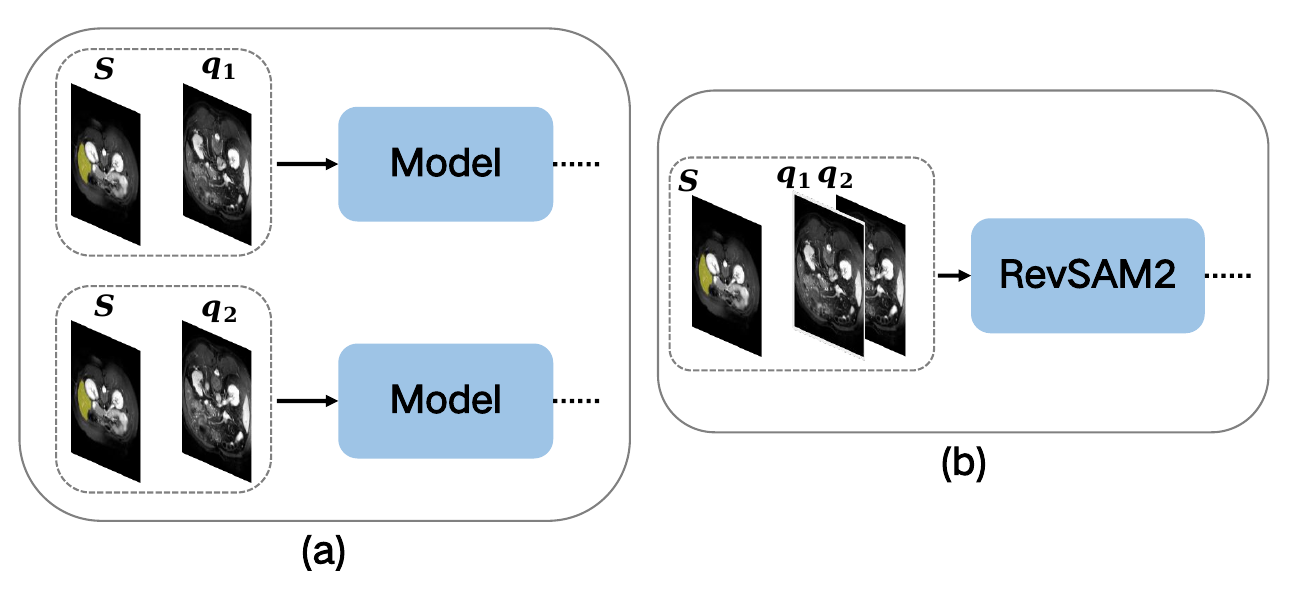}\vspace{-0.5em}
\caption{Comparison of the input pattern of other few-shot methods (a) with the input pattern of RevSAM2 (b).}
\label{fig:comp_few_shot}
\end{figure}

\vspace{-1em}
\section{Qualitative Results}\vspace{-1em}
\label{sec:qualitative}

\begin{figure*}[htbp]
    \centering
    \includegraphics[width=\linewidth]{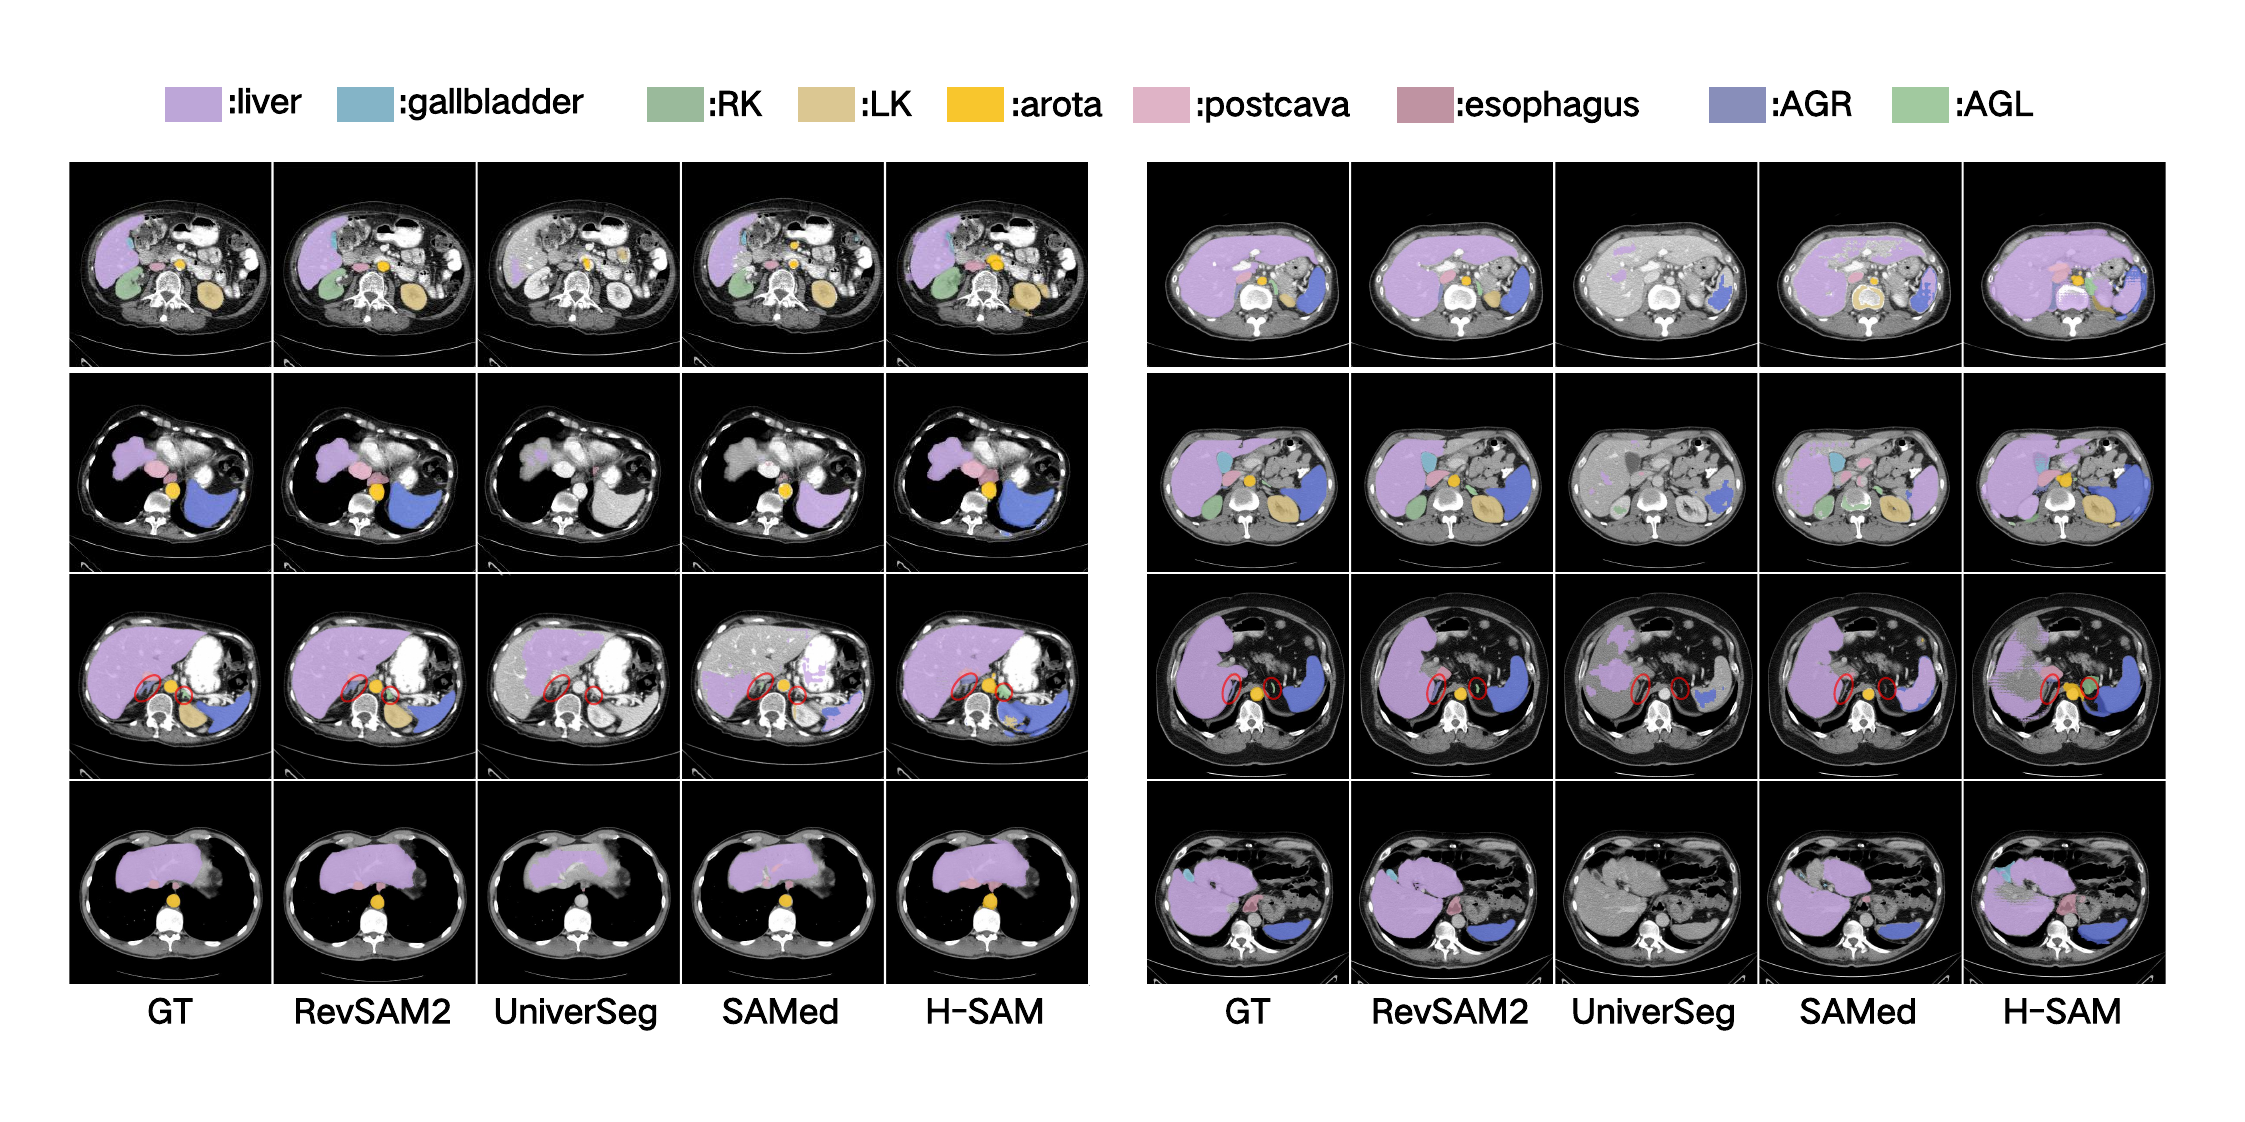}\vspace{-2em}
    \caption{The qualitative results of our RevSAM2 and other automatic segmentation methods, including UniverSeg, SAMed, and H-SAM (best viewed by zoom-in on screen) .}
    \label{fig:sup_compare_vis}
\end{figure*}

In Fig \ref{fig:sup_compare_vis} in the supplementary material, we provide a visual comparison with other prompt-free methods, \emph{i.e.}, UniverSeg \cite{universeg}, SAMed \cite{samed}, and H-SAM \cite{hsam}. For the low-resolution prediction mask of UniverSeg, we resize it to the original image size for display. From the results of SAMed and H-SAM, it can be seen that fine-tuning SAM with very few labels still makes it challenging to accurately identify the foreground region, leading to mis-segmentation. For UniverSeg, due to downscaling, edge details in the images are severely blurred, preventing it from producing high-quality masks. Compared to other methods, RevSAM2 generates the best predicted masks, particularly for small organs, such as the adrenal gland (AGR and AGL) in the third row, where only RevSAM2 correctly predicts it, highlight with a red circle on the third row in the figure.

\section{Reproducibility}
Our RevSAM2 is built upon SAM2 \footnote{https://github.com/facebookresearch/sam2}. The data split of BTCV and AbdomenCT follow CLIP-Driven Universal Model \footnote{https://github.com/ljwztc/CLIP-Driven-Universal-Model}, Synapse-CT and CHAOS-MRI follow RPT \footnote{https://github.com/YazhouZhu19/RPT} and GMRD \footnote{https://github.com/zmcheng9/GMRD}. Our code will be published after the paper is accepted.

\section{Detailed Results}
\label{sec:supp_detail_results}

In Table 1, 2 and 3 in main paper, we report the average results by using three groups of 10 support images for each organ compared with other methods. Here we report the detailed result of each group, termed as \textbf{Group-I}, \textbf{Group-II} and \textbf{Group-III}. It can be observed that the performance of other methods fluctuates significantly across different support images, particularly for the renew model approaches (nnU-Net, Swin UNETR). In some cases, when certain support images are used as the training set, these methods even fail to produce any valid segmentation results on the test set. For example, as shown in Table \ref{tab:BTCV dataset group 1} in the supplementary material, both nnU-Net and Swin UNETR fail to produce valid segmentation results when trained on the first group of 10 slices of the gallbladder on BTCV datset (see 0.00 in the 5th column in Table \ref{tab:BTCV dataset group 1} in the supplementary material). It is worth noting that RevSAM2's mDSC and mNSD substantially exceed the second-best metrics by a very large margin across all groups.

\begin{table*}[!htbp]

\centering
\resizebox{\linewidth}{!}
{
\begin{tabular}{c|cccccccccccccc|cc}
\toprule
Method             & spleen         & kidnetR        & kidneyL        & gall    & eso      & liver          & stomach        & arota          & IVC       & veins           & pancreas       & AG R           & AG L           & duode       & mDSC    &mNSD       \\ \midrule
nnU-Net \cite{nnunet}            & 21.19             & 29.55             & 35.42             & 0.00            & 14.06            & 31.27             & 12.17             & 32.77             & 14.68             & 16.72             & 15.35            & 0.00             & 19.31             & 8.14             & 17.90           & 15.34  \\
Swin UNETR \cite{swinunetr}         & 21.02             & 11.33             & 11.52             & 0.00            & 9.59             & 28.84             & 11.37             & 30.06             & 17.28             & 9.73             & 12.80             & 16.44             & 25.11             & 9.00             & 15.29           & 15.02  \\
UniverSeg \cite{universeg}          &65.11           & 64.45          &63.42           & 20.59          & 21.13          & 69.82          & 41.80          & 35.09          & 34.64          & 27.35          & 22.74          & 18.36          & 16.49          & 27.51        & 37.75        & 45.21  \\
SAMed \cite{samed}              & 70.36          & 51.00          & 56.33          & 45.11          & 35.36         & 78.97          & 38.01          & 69.21          & 38.98          & 33.53          & 25.67          & 6.31          & 13.40          & 18.23          & 41.46        & 35.72  \\
H-SAM \cite{hsam}              & {\ul 86.91}    & 75.82          & 77.61          & 65.99          & {\ul 51.66}          & {\ul 89.13}          & 54.88          & {\ul 78.76}          & 58.97          & 46.39          & 41.82          & {\ul 38.40}          & 31.97          & 38.62          & 59.78       & 51.76   \\
HQ-SAM \cite{hqsam}             & 74.60          & 66.37          & 77.32          & 53.73          & \textbf{66.65}           & 63.80          & 65.76          & 78.68          & {\ul 68.42}          & 23.59         & 49.45         & 29.52              &  \textbf{49.84}             & 39.85          & 57.68         &  51.43 \\
CAT-SAM \cite{catsam}            & 72.16          & 69.06       & {\ul 80.50}         & {\ul 70.46}          & 45.15          & 87.54          & {\ul 66.89}     & 61.51    & 66.75      & \textbf{64.65}         & {\ul 58.58}         & 32.78     & 38.28   & \textbf{50.78}     & {\ul 61.79}   &  {\ul 54.04} \\
MedicalSAM2 \cite{medicalsam2}           &   80.84         & {\ul 75.92}       & 68.01         & 55.03          & 38.58          & 83.89         & 66.72     & 31.78    & 53.50      & 26.36         & 45.58         & 33.08     & 9.51   & {\ul 46.16}     & 51.07   &  37.58 \\
RevSAM2(ours)   & \textbf{93.89}   & \textbf{81.13}    & \textbf{86.67}  & \textbf{83.05}    & 51.34 & \textbf{93.34} & \textbf{73.24} & \textbf{81.27} & \textbf{81.76} & {\ul 54.79}    & \textbf{63.69} & \textbf{52.72} & {\ul 48.78}    & 40.84  &\textbf{70.46} & \textbf{67.63}  \\ \bottomrule
\end{tabular}
}
\vspace{-0.5em}
\caption{Comparison of mDSC (\%) and mNSD (\%) on the BTCV dataset for support images \textbf{Group-I}.}\vspace{-1em}
\label{tab:BTCV dataset group 1}
\end{table*}

\begin{table*}[!htbp]

\centering
\resizebox{\linewidth}{!}
{
\begin{tabular}{c|ccccccccccccc|cc}
\toprule
Method             & liver          & kidneyR        & spleen         & pancreas       & arota          & IVC       & AGL            & AGR            & gall           & eso            & stomach        & duode       & kidneyL        & mDSC     &mNSD     \\ \midrule
nnU-Net \cite{nnunet}  &           66.95 &           76.44 &           81.65 &           25.74 &           59.12 &           56.48 &           23.54 &           33.11 &            8.99 &           17.46 &           21.13 &            6.13 &           74.08 &           42.37 &           29.85 \\
Swin UNETR \cite{swinunetr} &           19.88 &           25.06 &           54.83 &           21.16 &           33.48 &           43.12 &           27.34 &           12.76 &            0.00 &           22.99 &           16.16 &            0.00 &           55.39 &           25.55 &           21.90 \\
UniverSeg \cite{universeg} &           91.92 &           74.96 &           76.20 &           21.77 &           47.27 &           47.81 &           15.12 &           38.52 &           51.87 &           44.35 &           48.29 &           31.04 &           78.77 &           51.37 &           57.74 \\
SAMed \cite{samed} &           89.95 &           74.85 &           88.47 &           33.93 &           69.23 &           45.81 &           41.23 &           13.58 &           51.67 &           51.59 &           55.62 &           23.31 &           81.74 &           55.46 &           40.94 \\
H-SAM \cite{hsam}  &           84.11 & {\ul           95.43} &           87.83 &           48.57 & {\ul           82.36} &           76.82 & {\ul           55.43} & {\ul           49.43} &           72.11 &           49.34 &           81.64 &           38.22 & {\ul           92.96} & {\ul           70.33} & {\ul           59.02} \\
HQ-SAM \cite{hqsam} &           65.20 &           78.16 &           69.31 &            0.94 &           45.23 & \textbf{          87.40} &           47.34 &           24.14 &           67.04 & \textbf{          75.02} &           77.42 &           48.03 &           84.79 &           59.23 &           43.94 \\
CAT-SAM \cite{catsam} &           74.61 &           75.91 &           77.34 & \textbf{          67.80} &           60.73 &           61.44 &           37.06 &           33.58 &           61.89 &           54.53 & {\ul           82.94} & \textbf{          64.87} &           70.58 &           63.33 &           51.56 \\
MedicalSAM2 \cite{medicalsam2}  & {\ul           94.95} &           80.59 & {\ul           89.75} &           59.75 &           34.09 &           39.38 &           39.66 &           43.10 & {\ul           80.82} &           60.90 &           65.35 & {\ul           61.60} &           79.07 &           62.50 &           43.96 \\
RevSAM2(ours)      & \textbf{          96.64} & \textbf{          96.22} & \textbf{          96.90} & {\ul           64.80} & \textbf{          93.22} & {\ul           82.32} & \textbf{          65.03} & \textbf{          70.51} & \textbf{          85.71} & {\ul           74.66} & \textbf{          89.72} &           56.60 & \textbf{          95.82} & \textbf{          82.17} & \textbf{          77.18} \\ \bottomrule
\end{tabular}
}
\caption{Comparison of mDSC (\%) and mNSD (\%) on the AbdomenCT-1K dataset with other methods for support images \textbf{Group-I}.}
\label{tab:abdomenct group 1}
\end{table*}

\begin{table*}[!htbp]

\centering
\resizebox{\linewidth}{!}
{
\begin{tabular}{c|ccccccccccccc|c}
\toprule
Method             & spleen         & kidnetR        & kidneyL        & gall    & eso      & liver          & stomach        & arota          & IVC        & pancreas       & AG R           & AG L           & duode       & mDSC        \\ \midrule
UniverSeg \cite{universeg} &           75.02 &           68.18 &           70.45 &           33.13 &           26.29 & {\ul           87.20} &           51.17 &           42.15 &           48.59 &           31.45 &           20.71 &           13.66 &           31.86 &           46.14 \\
SAMed \cite{samed} &           73.41 &           55.80 &           45.31 &           40.23 &           24.46 &           86.91 &           33.82 &           69.49 &           41.30 &           14.86 &           34.72 &            1.09 &           11.74 &           41.01 \\
H-SAM \cite{hsam}  & {\ul           91.71} & {\ul           75.46} & {\ul           82.75} &           44.31 &           36.86 &           82.13 &           54.20 & {\ul           80.90} &           64.04 &           21.36 & {\ul           46.36} &           18.96 &           28.23 &           55.94 \\
HQ-SAM \cite{hqsam} &           71.41 &           72.01 &           77.50 & {\ul           63.52} & \textbf{          73.20} &           65.98 &           62.29 &           25.15 & \textbf{          84.69} &           46.63 & \textbf{          50.08} &            0.00 &           47.56 & {\ul           56.92} \\
CAT-SAM \cite{catsam} &           54.67 &           69.50 &           73.07 &           57.99 &           36.66 &           62.32 & \textbf{          75.17} &           45.91 &           52.98 & \textbf{          66.15} &           27.74 &            4.87 & \textbf{          61.54} &           52.97 \\
MedicalSAM2 \cite{medicalsam2}  &           84.72 &           74.86 &           65.52 &           49.74 &           41.38 &           69.94 &           60.57 &           24.29 &           38.97 & {\ul           47.99} &           30.78 & {\ul           26.06} & {\ul           52.64} &           51.34 \\
RevSAM2(ours)      & \textbf{          94.87} & \textbf{          83.75} & \textbf{          83.76} & \textbf{          74.80} & {\ul           56.22} & \textbf{          93.34} & {\ul           71.19} & \textbf{          85.28} & {\ul           77.11} &           47.66 &           27.03 & \textbf{          38.73} &           43.80 & \textbf{          67.50} \\ \bottomrule
\end{tabular}
}
\caption{Domain adaptation comparison of mDSC (\%) on the BTCV dataset using support images \textbf{Group-I} of AbdomenCT-1K.}
\label{tab:BTCV AbdomenCT-group 1}
\end{table*}

\begin{table*}[!htbp]

\centering
\resizebox{\linewidth}{!}
{
\begin{tabular}{c|ccccccccccccc|c}
\toprule
Method             & liver & kidneyR & spleen & pancreas & arota & IVC & AGL & AGR & gall & eso & stomach & duode & kidneyL & mDSC \\ \midrule
UniverSeg \cite{universeg} &           92.08 &           77.08 &           75.27 &           42.79 &           58.48 &           52.02 &           23.18 &           18.91 &           29.97 &           33.17 &           39.22 &           23.85 &           81.61 &           49.82 \\
SAMed \cite{samed} &           88.62 &           59.83 &           60.71 &           21.58 &           59.86 &           44.68 &            2.85 &           17.14 &           58.66 &           37.84 &           17.15 &           28.45 &           66.16 &           43.35 \\
H-SAM \cite{hsam}  &           92.54 & {\ul           92.95} & {\ul           88.51} &           48.75 &           77.38 & {\ul           70.01} &           12.58 & \textbf{          64.82} &           76.10 &           58.77 &           43.74 &           42.31 & {\ul           89.38} &           65.99 \\
HQ-SAM \cite{hqsam} &           36.55 &           65.42 &           73.09 & {\ul           58.90} & {\ul           90.04} & \textbf{          73.31} &            0.00 &           31.35 &           55.06 & \textbf{          68.82} &           75.62 &           41.44 &           81.64 &           57.79 \\
CAT-SAM \cite{catsam} &           89.26 &           84.90 &           81.08 & \textbf{          67.15} &           73.49 &           60.54 & {\ul           52.99} &           45.96 &           71.98 &           59.22 & {\ul           77.05} & \textbf{          53.80} &           74.82 & {\ul           68.63} \\
MedicalSAM2 \cite{medicalsam2}  & \textbf{          93.49} &           92.41 &           79.22 &           55.87 &           56.36 &           58.29 &           37.70 &           40.62 & {\ul           81.75} &           60.71 &           55.28 & {\ul           52.32} &           84.48 &           65.27 \\
RevSAM2(ours)      & {\ul           93.40} & \textbf{          95.07} & \textbf{          96.71} &           54.64 & \textbf{          93.30} &           64.56 & \textbf{          60.10} & {\ul           55.22} & \textbf{          83.23} & {\ul           65.26} & \textbf{          86.89} &           46.17 & \textbf{          95.44} & \textbf{          76.15} \\\bottomrule
\end{tabular}
}
\caption{Domain adaptation comparison of mDSC (\%) on the AbdomenCT-1K dataset using support images \textbf{Group-I} of BTCV.}
\label{tab:AbdomenCT BTCV-group 1}
\end{table*}

\begin{table*}[!htbp]

\centering
\resizebox{\linewidth}{!}
{
\begin{tabular}{c|cccccccccccccc|cc}
\toprule
Method             & spleen         & kidnetR        & kidneyL        & gall    & eso      & liver          & stomach        & arota          & IVC       & veins           & pancreas       & AG R           & AG L           & duode       & mDSC    &mNSD       \\ \midrule
nnU-Net \cite{nnunet}  &           15.78 &           26.13 &           41.60 &           22.98 &            6.75 &            9.93 &           11.62 &           38.95 &            8.74 &           11.48 &           22.13 &            7.52 &            0.00 &            7.78 &           16.53 &           16.55 \\
Swin UNETR \cite{swinunetr} &           30.16 &           25.30 &           13.69 &           18.97 &           10.30 &           30.71 &           11.99 &           26.37 &           12.12 &            6.77 &           22.22 &            5.50 &           17.64 &            9.27 &           17.21 &           14.41 \\
UniverSeg \cite{universeg} &           49.58 &           64.52 &           66.47 &           21.27 &           23.70 &           80.35 &           38.48 &           59.07 &           28.15 &           25.06 &           16.14 &            6.15 &            4.76 &           18.46 &           35.87 &           42.38 \\
SAMed \cite{samed} &           68.55 &           46.15 &           37.61 &           31.36 &           37.96 & {\ul           87.76} &           37.60 &           63.84 &           30.25 &           43.42 &           19.45 &            5.32 &            1.66 &           10.29 &           37.23 &           32.98 \\
H-SAM \cite{hsam}  & {\ul           90.55} & {\ul           75.59} & {\ul           80.87} &           45.17 &           50.02 &           87.43 &           47.59 & {\ul           82.55} &           52.08 &           49.39 &           17.42 &           32.37 &           30.15 &           19.03 &           54.30 &           50.49 \\
HQ-SAM \cite{hqsam} &           73.81 &           68.95 &           76.48 & {\ul           74.91} & \textbf{          79.90} &           69.66 &           61.15 &           61.45 & {\ul           75.49} &            6.78 &           45.82 &           32.02 & \textbf{          49.91} &           37.55 &           58.13 &           50.09 \\
CAT-SAM \cite{catsam} &           67.92 &           33.35 &           72.06 &           53.63 &           54.87 &           86.53 & \textbf{          75.35} &           65.39 &           62.01 & \textbf{          60.91} & \textbf{          61.56} &           28.48 &           36.61 & \textbf{          64.30} & {\ul           58.78} & {\ul           54.94} \\
MedicalSAM2 \cite{medicalsam2}  &           79.16 &           72.52 &           71.09 &           58.88 &           55.05 &           85.87 &           50.49 &           30.46 &           49.00 &           23.35 &           45.54 & {\ul           34.19} &           24.97 &           39.83 &           51.46 &           37.64 \\
RevSAM2(ours)      & \textbf{          94.55} & \textbf{          85.23} & \textbf{          85.52} & \textbf{          79.22} & {\ul           58.58} & \textbf{          92.14} & {\ul           72.09} & \textbf{          88.47} & \textbf{          78.78} & {\ul           59.52} & {\ul           51.53} & \textbf{          41.39} & {\ul           36.71} & {\ul           43.90} & \textbf{          69.12} & \textbf{          67.50} \\ \bottomrule
\end{tabular}
}
\caption{Comparison of mDSC (\%) and mNSD (\%) on the BTCV dataset for support images \textbf{Group-II}.}
\label{tab:BTCV dataset group 2}
\end{table*}

\begin{table*}[!htbp]

\centering
\resizebox{\linewidth}{!}
{
\begin{tabular}{c|ccccccccccccc|cc}
\toprule
Method             & liver & kidneyR & spleen & pancreas & arota & IVC & AGL & AGR & gall & eso & stomach & duode & kidneyL & mDSC & mNSD \\ \midrule
nnU-Net \cite{nnunet}  &           79.62 &           72.31 &           34.94 &           25.71 &           59.09 &           63.26 &           11.74 &           43.68 &           22.60 &           29.83 &            6.43 &           14.52 &           73.83 &           41.35 &           33.09 \\
Swin UNETR \cite{swinunetr} &           75.70 &           50.80 &           52.79 &           28.70 &           45.64 &           34.58 &           28.80 &           34.10 &           27.99 &           24.45 &            9.36 &            0.00 &           54.32 &           35.94 &           26.77 \\
UniverSeg \cite{universeg} &           86.49 &           75.20 &           79.73 &           25.43 &           63.16 &           47.53 &           28.68 &           23.70 &           27.30 &           33.87 &           57.30 &           31.86 &           75.46 &           50.44 &           55.89 \\
SAMed \cite{samed} &           86.84 &           71.51 &           56.33 &           36.84 &           72.89 &           19.84 &           35.01 &            3.50 &           59.37 &           53.52 &           33.64 &           20.91 &           80.06 &           48.48 &           34.95 \\
H-SAM \cite{hsam}  &           92.74 & {\ul           94.56} & {\ul           90.05} &           51.20 & {\ul           83.25} &           69.04 & {\ul           60.09} &           23.67 &           60.04 &           56.10 &           70.49 &           44.28 & {\ul           91.53} &           68.23 &           56.80 \\
HQ-SAM \cite{hqsam} &           74.20 &           52.16 &           73.62 &           57.52 &           78.26 & \textbf{          81.86} &           42.06 &            2.31 &           71.54 &           49.95 &           69.88 &           45.63 &           74.50 &           59.50 &           39.12 \\
CAT-SAM \cite{catsam} &           89.63 &           84.45 &           77.16 & {\ul           64.88} &           72.75 &           65.42 &           45.25 & {\ul           50.73} &           69.97 & {\ul           62.15} &           78.63 & \textbf{          58.76} &           84.33 & {\ul           69.55} & {\ul           56.84} \\
MedicalSAM2 \cite{medicalsam2}  & \textbf{          95.90} &           77.95 &           89.06 &           58.71 &           20.93 &           66.60 &           46.14 &           35.36 & {\ul           76.81} &           59.51 & {\ul           80.28} & {\ul           56.97} &           85.94 &           65.40 &           45.17 \\
RevSAM2(ours)      & {\ul           95.68} & \textbf{          96.23} & \textbf{          97.07} & \textbf{          69.42} & \textbf{          93.62} & {\ul           81.66} & \textbf{          68.91} & \textbf{          70.82} & \textbf{          81.40} & \textbf{          74.45} & \textbf{          91.74} &           54.40 & \textbf{          95.66} & \textbf{          82.39} & \textbf{          77.19} \\ \bottomrule
\end{tabular}
}
\caption{Comparison of mDSC (\%) and mNSD (\%) on the AbdomenCT-1K dataset with other methods for support images \textbf{Group-II}.}
\label{tab:abdomenct dataset group 2}
\end{table*}

\begin{table*}[!htbp]

\centering
\resizebox{\linewidth}{!}
{
\begin{tabular}{c|ccccccccccccc|c}
\toprule
Method             & spleen         & kidnetR        & kidneyL        & gall    & eso      & liver          & stomach        & arota          & IVC        & pancreas       & AG R           & AG L           & duode       & mDSC        \\ \midrule
UniverSeg \cite{universeg} &           78.41 &           71.63 &           63.55 &           30.59 &           31.59 &           83.24 &           38.60 &           50.44 &           40.50 &           35.34 &            3.71 &            7.89 &           30.51 &           43.54 \\
SAMed \cite{samed} &           70.60 &           41.25 &           59.31 &           30.96 &           28.23 &           84.03 &           21.44 &           69.35 &           26.88 &           28.46 &           24.87 &            1.49 &           12.71 &           38.43 \\
H-SAM \cite{hsam}  & {\ul           85.66} &           72.54 &           73.84 &           40.20 &           37.42 & {\ul           90.80} &           32.12 &           77.40 &           65.44 &           40.90 & {\ul           44.97} &           16.56 &           32.98 &           54.68 \\
HQ-SAM \cite{hqsam} &           65.91 &           73.49 &           74.72 & {\ul           70.26} & \textbf{          68.22} &           60.96 &           55.10 & {\ul           79.98} & {\ul           79.28} &           46.26 &           41.22 &           21.79 & {\ul           49.57} &           60.52 \\
CAT-SAM \cite{catsam} &           50.41 & {\ul           79.63} &           77.91 &           60.89 & {\ul           58.38} &           87.79 & {\ul           68.91} &           68.00 &           66.01 & {\ul           53.96} & \textbf{          46.63} & \textbf{          45.27} & \textbf{          51.25} & {\ul           62.70} \\
MedicalSAM2 \cite{medicalsam2}  &           69.31 &           67.34 & {\ul           82.07} &           56.72 &           48.75 &           72.36 &           67.24 &           26.65 &           59.84 &           47.79 &           35.44 &           26.57 &           48.01 &           54.47 \\
RevSAM2(ours)      & \textbf{          95.02} & \textbf{          83.86} & \textbf{          86.00} & \textbf{          72.18} &           53.43 & \textbf{          93.79} & \textbf{          73.50} & \textbf{          87.89} & \textbf{          80.33} & \textbf{          54.25} &           44.74 & {\ul           42.80} &           46.86 & \textbf{          70.36} \\ \bottomrule
\end{tabular}
}
\caption{Domain adaptation comparison of mDSC (\%) on the BTCV dataset using support images \textbf{Group-II} of AbdomenCT-1K.}
\label{tab:BTCV ABdomenCT-group 2}
\end{table*}

\begin{table*}[!htbp]

\centering
\resizebox{\linewidth}{!}
{
\begin{tabular}{c|ccccccccccccc|c}
\toprule
Method             & liver & kidneyR & spleen & pancreas & arota & IVC & AGL & AGR & gall & eso & stomach & duode & kidneyL & mDSC \\ \midrule
UniverSeg \cite{universeg} &           90.57 &           90.32 &           83.88 &           28.51 &           66.73 &           41.45 &            8.26 &           34.10 &           54.51 &           37.85 &           65.75 &           29.54 &           83.42 &           54.99 \\
SAMed \cite{samed} &           91.93 &           80.81 &           83.34 &           43.87 &           63.31 &           31.50 &           19.20 &            5.98 &           51.59 &           47.46 &           60.83 &            8.12 &           65.58 &           50.27 \\
H-SAM \cite{hsam}  &           91.50 &           93.29 & {\ul           96.42} &           29.13 & {\ul           81.13} &           58.71 &           42.97 & {\ul           48.86} &           53.05 & {\ul           69.68} &           62.50 &           16.74 & {\ul           91.50} &           64.27 \\
HQ-SAM \cite{hqsam} &           53.95 &           76.11 &           72.52 &           56.55 &           76.28 & {\ul           80.44} &           47.10 &           34.92 &           73.75 & \textbf{          88.72} &           72.23 &           38.06 &           80.08 &           65.44 \\
CAT-SAM \cite{catsam} &           89.17 &           69.83 &           72.22 & \textbf{          67.81} &           76.79 &           67.20 & {\ul           55.93} &           42.51 &           68.47 &           59.09 & \textbf{          83.43} & \textbf{          66.23} &           82.85 & {\ul           69.35} \\
MedicalSAM2 \cite{medicalsam2}  & \textbf{          94.80} & {\ul           93.61} &           85.39 & {\ul           60.20} &           54.45 &           48.61 &           35.17 &           43.25 & {\ul           80.36} &           64.72 &           65.36 & {\ul           52.77} &           72.58 &           65.48 \\
RevSAM2(ours)      & {\ul           92.93} & \textbf{          95.37} & \textbf{          96.96} &           53.90 & \textbf{          93.83} & \textbf{          81.16} & \textbf{          67.15} & \textbf{          73.27} & \textbf{          87.08} &           55.50 & {\ul           78.28} &           34.27 & \textbf{          95.40} & \textbf{          77.31} \\\bottomrule
\end{tabular}
}
\caption{Domain adaptation comparison of mDSC (\%) on the AbdomenCT-1K dataset using support images \textbf{Group-II} of BTCV.}
\label{tab:AbdomenCT BTCV-group 2}
\end{table*}

\begin{table*}[!htbp]

\centering
\resizebox{\linewidth}{!}
{
\begin{tabular}{c|cccccccccccccc|cc}
\toprule
Method             & spleen         & kidnetR        & kidneyL        & gall    & eso      & liver          & stomach        & arota          & IVC       & veins           & pancreas       & AG R           & AG L           & duode       & mDSC    &mNSD       \\ \midrule
nnU-Net \cite{nnunet}  &           17.04 &           20.51 &           14.78 &            0.00 &            9.99 &           56.27 &           13.19 &           35.83 &           18.77 &            6.24 &           17.91 &            6.72 &           16.41 &            9.50 &           17.37 &           16.65 \\
Swin UNETR \cite{swinunetr} &           11.53 &           23.14 &            0.00 &            0.00 &           24.49 &           41.13 &           12.06 &           28.72 &           19.06 &            0.00 &           12.74 &            0.00 &           23.09 &           16.07 &           15.14 &           13.08 \\
UniverSeg \cite{universeg} &           62.16 &           66.79 &           63.31 &           31.42 &           23.64 &           81.12 &           44.56 &           46.93 &           44.78 &           30.45 &           26.37 &           22.16 &           15.57 &            7.36 &           40.47 &           48.43 \\
SAMed \cite{samed} &           75.86 &           44.17 &           63.98 &           19.01 &           23.75 &           85.35 &           45.30 &           64.94 &           39.94 &           34.76 &           29.76 &            3.35 &            9.06 &           17.74 &           39.78 &           32.85 \\
H-SAM \cite{hsam}  & {\ul           86.33} &           72.82 & \textbf{          87.38} & {\ul           56.08} &           34.57 & {\ul           92.54} &           62.70 & {\ul           78.97} &           47.38 &           32.27 &           27.15 &           19.13 &           33.04 &           21.87 &           53.73 &           49.56 \\
HQ-SAM \cite{hqsam} &           75.21 & {\ul           73.31} &           68.10 &           52.41 & \textbf{          75.59} &           68.76 &           63.22 &           48.79 & \textbf{          82.46} &           12.05 &           45.65 & {\ul           46.48} & \textbf{          55.65} &           45.50 &           58.08 &           43.72 \\
CAT-SAM \cite{catsam} &           77.52 &           54.36 &           29.62 &           52.82 &           53.36 &           87.92 & \textbf{          82.99} &           63.97 &           66.43 & \textbf{          59.01} & \textbf{          59.66} &           31.33 &           49.81 & \textbf{          56.17} & {\ul           58.93} & {\ul           57.39} \\
MedicalSAM2 \cite{medicalsam2}  &           75.98 &           73.25 &           70.46 &           54.48 &           41.63 &           86.72 & {\ul           67.69} &           28.30 &           48.96 &           32.24 &           46.12 &           31.83 &           35.79 & {\ul           53.22} &           53.33 &           40.61 \\
RevSAM2(ours)      & \textbf{          93.53} & \textbf{          81.15} & {\ul           85.15} & \textbf{          81.28} & {\ul           56.36} & \textbf{          93.06} &           66.76 & \textbf{          88.47} & {\ul           74.10} & {\ul           50.43} & {\ul           58.65} & \textbf{          56.75} & {\ul           50.17} &           44.17 & \textbf{          70.00} & \textbf{          67.86} \\ \bottomrule
\end{tabular}
}
\vspace{-0.5em}
\caption{Comparison of mDSC (\%) and mNSD (\%) on the BTCV dataset for support images \textbf{Group-III}.}
\label{tab:BTCV dataset group 3}
\end{table*}

\begin{table*}[!htbp]

\centering
\resizebox{\linewidth}{!}
{
\begin{tabular}{c|ccccccccccccc|cc}
\toprule
Method             & liver & kidneyR & spleen & pancreas & arota & IVC & AGL & AGR & gall & eso & stomach & duode & kidneyL & mDSC & mNSD \\ \midrule
nnU-Net \cite{nnunet}  &           68.00 &           79.91 &           46.21 &           21.63 &           65.84 &           52.59 &           28.35 &           19.07 &            7.12 &           29.89 &            7.91 &           13.94 &           56.10 &           38.20 &           26.07 \\
Swin UNETR \cite{swinunetr} &           65.95 &           53.68 &           52.69 &           15.77 &           45.61 &           17.33 &           28.73 &            0.00 &           14.08 &           21.64 &           11.13 &           17.81 &           35.74 &           29.24 &           21.34 \\
UniverSeg \cite{universeg} &           90.12 &           83.42 &           77.69 &           40.67 &           65.36 &           55.14 &           26.68 &           24.80 &           37.77 &           56.13 &           64.84 &           37.80 &           76.88 &           56.72 & {\ul           61.79} \\
SAMed \cite{samed} &           91.76 &           76.73 &           64.62 &           43.31 &           64.46 &           40.87 &           30.90 &           17.03 &           70.46 &           64.90 &           56.73 &           32.26 &           76.11 &           56.16 &           41.71 \\
H-SAM \cite{hsam}  &           94.12 & {\ul           91.29} & {\ul           95.56} &           53.98 &           72.62 &           64.07 & {\ul           48.77} &           54.20 & {\ul           81.05} &           72.03 &           70.78 &           49.68 & {\ul           91.51} & {\ul           72.28} &           60.21 \\
HQ-SAM \cite{hqsam} &           74.12 &           76.55 &           70.20 &           60.16 & {\ul           83.82} & \textbf{          85.02} &           38.55 &            0.14 &           64.04 & \textbf{          78.76} &           63.62 &           46.48 &           81.39 &           63.30 &           44.58 \\
CAT-SAM \cite{catsam} &           90.49 &           86.16 &           86.62 & {\ul           67.61} &           69.25 &           68.57 &           43.56 & {\ul           56.85} &           71.56 &           62.17 & {\ul           81.96} & \textbf{          60.04} &           87.87 &           71.75 &           60.45 \\
MedicalSAM2 \cite{medicalsam2}  & \textbf{          94.70} &           69.74 &           92.90 &           60.35 &           32.57 &           58.90 &           44.03 &           43.00 &           80.43 &           66.08 &           78.42 & {\ul           58.84} &           73.12 &           65.62 &           43.04 \\
RevSAM2(ours)      & {\ul           94.15} & \textbf{          96.23} & \textbf{          97.23} & \textbf{          72.54} & \textbf{          92.65} & {\ul           81.35} & \textbf{          69.02} & \textbf{          73.26} & \textbf{          84.28} & {\ul           76.84} & \textbf{          90.76} &           53.54 & \textbf{          94.95} & \textbf{          82.83} & \textbf{          77.63} \\ \bottomrule
\end{tabular}
}
\caption{Comparison of mDSC (\%) and mNSD (\%) on the AbdomenCT-1K dataset with other methods for support images \textbf{Group-III}.}
\label{tab:abdomenct dataset group 3}
\end{table*}

\begin{table*}[!htbp]

\centering
\resizebox{\linewidth}{!}
{
\begin{tabular}{c|ccccccccccccc|c}
\toprule
Method             & spleen         & kidnetR        & kidneyL        & gall    & eso      & liver          & stomach        & arota          & IVC        & pancreas       & AG R           & AG L           & duode       & mDSC        \\ \midrule
UniverSeg \cite{universeg} &           77.28 &           66.03 &           70.36 &           34.14 &           26.38 &           85.76 &           50.71 &           36.08 &           46.43 &           31.09 &            6.95 &           10.45 &           28.99 &           43.90 \\
SAMed \cite{samed} &           67.68 &           62.37 &           37.62 &           48.63 &           35.86 &           87.23 &           46.06 &           62.30 &           38.53 &           26.78 &           21.71 &            8.52 &           12.68 &           42.77 \\
H-SAM \cite{hsam}  & {\ul           91.29} &           71.97 & {\ul           85.00} &           53.33 &           43.07 & {\ul           90.89} &           47.60 &           74.51 &           48.09 &           24.22 &           33.05 &           19.66 &           25.75 &           54.50 \\
HQ-SAM \cite{hqsam} &           65.91 &           76.55 &           74.72 & \textbf{          70.26} & \textbf{          68.22} &           65.58 &           55.10 & {\ul           79.98} & \textbf{          79.28} &           46.26 & \textbf{          41.22} &           21.79 &           49.57 &           61.11 \\
CAT-SAM \cite{catsam} &           69.09 & {\ul           80.14} & \textbf{          85.31} &           51.85 &           52.38 &           87.94 & {\ul           69.78} &           52.97 &           67.34 & \textbf{          59.88} &           30.37 & \textbf{          46.81} & \textbf{          63.22} & {\ul           62.85} \\
MedicalSAM2 \cite{medicalsam2}  &           82.65 &           71.65 &           74.56 &           60.97 &           48.48 &           77.37 &           65.11 &           34.05 &           52.24 &           49.85 &           34.76 &           29.53 & {\ul           53.20} &           56.49 \\
RevSAM2(ours)      & \textbf{          94.83} & \textbf{          81.41} &           84.19 & {\ul           65.55} & {\ul           60.13} & \textbf{          93.96} & \textbf{          73.68} & \textbf{          87.68} & {\ul           78.87} & {\ul           58.30} & {\ul           39.36} & {\ul           32.95} &           49.10 & \textbf{          69.23} \\ \bottomrule
\end{tabular}
}
\caption{Domain adaptation comparison of mDSC (\%) on the BTCV dataset using support images \textbf{Group-III} of AbdomenCT-1K.}
\label{tab:BTCV AbdomenCT-group 3}
\end{table*}

\begin{table*}[!htbp]

\centering
\resizebox{\linewidth}{!}
{
\begin{tabular}{c|ccccccccccccc|c}
\toprule
Method             & liver & kidneyR & spleen & pancreas & arota & IVC & AGL & AGR & gall & eso & stomach & duode & kidneyL & mDSC \\ \midrule
UniverSeg \cite{universeg} &           88.74 &           87.82 &           52.92 &           51.52 &           52.51 &           59.30 &           21.87 &           31.50 &           49.67 &           39.60 &           33.34 &           34.19 &           81.75 &           52.67 \\
SAMed \cite{samed} &           89.68 &           67.80 &           72.81 &           24.83 &           51.59 &           33.41 &            0.09 &            3.90 &           17.45 &           34.53 &           46.06 &           16.91 &           69.63 &           40.67 \\
H-SAM \cite{hsam}  &           93.49 & {\ul           88.67} & {\ul           83.03} &           27.71 &           69.11 &           42.89 &           23.06 &           37.11 &           72.86 &           45.01 &           63.83 &           25.75 & {\ul           92.67} &           58.86 \\
HQ-SAM \cite{hqsam} &           57.73 &           65.10 &           76.73 &           56.53 &           66.15 & \textbf{          83.26} &           50.73 &            0.00 &            0.00 & \textbf{          83.55} &           62.90 &           42.69 &           68.88 &           54.94 \\
CAT-SAM \cite{catsam} &           89.94 &           86.25 &           80.40 &           60.51 & {\ul           73.33} &           63.82 & {\ul           54.21} &           46.57 &           72.85 & {\ul           60.72} & {\ul           75.01} & \textbf{          58.06} &           40.55 & {\ul           66.32} \\
MedicalSAM2 \cite{medicalsam2}  & \textbf{          94.30} &           78.69 &           81.42 & {\ul           62.12} &           64.05 &           35.89 &           37.67 & {\ul           56.03} & {\ul           78.76} &           59.61 &           69.62 & {\ul           56.70} &           70.69 &           65.04 \\
RevSAM2(ours)      & {\ul           93.89} & \textbf{          95.71} & \textbf{          96.68} & \textbf{          68.36} & \textbf{          93.40} & {\ul           79.41} & \textbf{          68.04} & \textbf{          64.03} & \textbf{          84.82} &           59.66 & \textbf{          75.98} &           51.24 & \textbf{          95.20} & \textbf{          78.96} \\\bottomrule
\end{tabular}
}
\caption{Domain adaptation comparison of mDSC (\%) on the AbdomenCT-1K dataset using support images \textbf{Group-III} of BTCV.}
\label{tab:AbdomenCT BTCV-group 3}
\end{table*}
